# Supplementary material for: DeltaGrad: Rapid retraining of machine learning models
Source: arXiv:2006.14755 source file (2020-06-30)
Supplement: Supplementary file 1 [file Appendix.tex]

\section{Appendix}

\subsection{How to select parameters}

% \begin{figure}[ht]
% % \vskip 0.2in
% \begin{center}
% \centerline{\includegraphics[width=0.8\columnwidth]{Figures/MNIST_deletion/incremental_varied_periods_4096_0.00002_20.png}}
% \caption{Running time and Distance over \MNIST\ with one sample removed, period = 10}
% \label{fig: varied_deletion_rate_20_10}
% \centerline{\includegraphics[width=0.8\columnwidth]{Figures/MNIST_deletion/incremental_varied_inits_4096_0.00002_5.png}}
% \caption{Running time and Distance over \MNIST\ with one sample removed, period = 5}
% \label{fig: varied_deletion_rate_20_5}
% \end{center}
% % \vskip -0.2in
% \end{figure}
